# Supplementary material for: Sadeed: Advancing Arabic Diacritization Through Small Language Model
Source: arXiv:2504.21635 source file (2025-08-21)
Supplement: Supplementary file 1 [file table_1.pdf]

| Sample                                                                                                                                                                                                                                                                                                                                                                                                                                                                                                                                                                 | Translation                                                                                                                                                                                                                                                                                                                                                                                                                                                                                                                  | Source   |
|------------------------------------------------------------------------------------------------------------------------------------------------------------------------------------------------------------------------------------------------------------------------------------------------------------------------------------------------------------------------------------------------------------------------------------------------------------------------------------------------------------------------------------------------------------------------|------------------------------------------------------------------------------------------------------------------------------------------------------------------------------------------------------------------------------------------------------------------------------------------------------------------------------------------------------------------------------------------------------------------------------------------------------------------------------------------------------------------------------|----------|
| تَقُولُ أَنَّ فَادِيمَانَ فِي مُقَدِّمَةِ كِتَابِهَا «مِنْ كُتُبِي: اعْتِرَافَاتُ قَارِئَةٍ عَادِيَةٍ» أَنَّ الْكُتُبَ، حَتَّى تِلْكَ الَّتِي نُشِرَتْ قَبْلَ وَلَادَتِهَا، لَا تَشِيخُ، بَلْ تَظَلُّ شَاهِدَةً عَلَى مُرُورِ الزَّمَنِ، تَذَكِّرُنَا بِالْأَوْقَاتِ الَّتِي قَرَأْنَاهَا فِيهَا أَوْ أَعَدْنَا قِرَاءَتَهَا، تَقِفُ أَمَامَنَا كَمِرَآةٍ تَعَكِّسُ عُقُودًا مَضَتْ، هَكَذَا أَنْظَرُ إِلَى مَكْتَبَتِي، كَمَا يَنْظُرُ الرَّفِيقُ إِلَى رَفِيقِهِ،                                                                                                    | Ann Fadiman says in the introduction of her book "Confessions of an Ordinary Reader" that books, even those published before our birth, do not age, but rather remain a witness to the passage of time, reminding us of the moments in which we read them or re-read them, standing before us like a mirror reflecting decades past; this is how I look at my library, just as a companion looks at their companion.                                                                                                         | Our      |
| حَبَّتَانِ بَطَاطِسَ كَبِيرَتَانِ. زَيْتٌ نَبَاتِيٌّ لَلْقَلِي. مِلْحٌ وَفَلْفَلٌ أَسْوَدٌ حَسَبَ الرِّغْبَةِ. لَيُونٌ لِلتَّقْدِيمِ. مُكَوَّنَاتٌ صُلْبَةٌ التَّارْتَارِ: نَصْفُ كُوبٍ مَائُونِيز. مِلْعَقَةٌ كَبِيرَةٌ مِنْ مَخْلَلِ خِيَارٍ مَفْرُومٍ نَاعِمٍ. مِلْعَقَةٌ كَبِيرَةٌ مِنْ شَبِثٍ مَفْرُومٍ نَاعِمٍ. مِلْعَقَةٌ صَغِيرَةٌ مِنْ عَصِيرِ لَيُونٍ طَارِجٍ. مِلْعَقَةٌ صَغِيرَةٌ مِنْ خَرْدَلٍ دِيْجُونٍ. نَصْفُ مِلْعَقَةٍ صَغِيرَةٍ مِنَ السُّكَّرِ. مِلْحٌ وَفَلْفَلٌ أَسْوَدٌ حَسَبَ الرِّغْبَةِ.                                                     | 2 large potatoes Vegetable oil for frying Salt and black pepper to taste Lemon for serving<br>Tartar Sauce Ingredients: 1/2 cup mayonnaise 1 large tablespoon finely chopped pickles 1 large tablespoon finely chopped dill 1 small teaspoon fresh lemon juice 1 small teaspoon Dijon mustard 1/2 small teaspoon sugar Salt and black pepper to taste                                                                                                                                                                        | Our      |
| تُعَدُّ نَظَرِيَّةُ الضُّغُوطِ (yroeHT niartS) إِحْدَى النِّظَرِيَّاتِ الْبَارِزَةِ فِي عِلْمِ الْجَرِيمَةِ، الَّتِي تُقَدِّمُ تَفْسِيرًا لِكَيْفِيَّةِ نَشُوءِ السُّلُوكِ الْأَجْرَائِيِّ. وَفَقًا لِهَذِهِ النِّظَرِيَّةِ، فَإِنَّ الْأَفْرَادَ الَّذِينَ يُوَجِّهُونَ ضُغُوطًا اجْتِمَاعِيَّةً واِقْتِصَادِيَّةً شَدِيدَةً مِثْلَ الْفَقْرِ، أَوْ عَدَمِ الْقُدْرَةِ عَلَى تَحْقِيقِ أَهْدَافِهِمُ الْمَشْرُوعَةِ مِنْ خِلَالِ الْوَسَائِلِ التَّقْلِيدِيَّةِ، قَدْ يَلْجَأُونَ إِلَى سُلُوكِيَّاتٍ إِجْرَامِيَّةٍ كَوَسِيلَةٍ لِلتَّكْيُفِ مَعَ هَذِهِ الضُّغُوطِ. | The Strain Theory is one of the prominent theories in criminology that provides an explanation for the emergence of criminal behavior. According to this theory, individuals who face severe social and economic pressures, such as poverty or the inability to achieve their legitimate goals through traditional means, may resort to criminal behaviors as a way of adapting to these pressures.                                                                                                                          | Our      |
| مَنْ كَانَ لَمْ يُؤْتِ عِلْمًا فِي بَقَاءِ غَدٍ مَاذَا تَفَكَّرُهُ فِي رِزْقٍ بَعْدَ غَدٍ يَا وَاعِظَ النَّاسِ عَمَّا أَنْتَ فَاعِلُهُ يَا مَنْ يَدُّ عَلَيْهِ الْعُمُرُ بِالنَّفْسِ احْفَظْ لَشَبِيكَ مِنْ عَيْبٍ يَدْنِسُهُ إِنَّ الْبَيَاضَ قَلِيلٌ الْحَمَلُ لِلدَّنَسِ كَحَامِلٍ لِثِيَابِ النَّاسِ يَغْسِلُهَا وَثُبُهُ غَارِقٌ فِي الرَّجْسِ وَالنَّجَسِ تَبْغِي النِّجَاةَ وَلَمْ تَسْلُكْ طَرِيقَهَا إِنَّ السَّفِينَةَ لَا تَجْرِي عَلَى الْيَبْسِ                                                                                                           | Who has not been granted knowledge about the survival of tomorrow, Why do you ponder the sustenance of the day after tomorrow, O preacher of people What will you do, O you whose life is counted by breaths? Preserve your gray hair from a disgrace that might taint it, Indeed, whiteness has little tolerance for impurity. Like one who washes people's clothes While his own garment is drowning in filth and uncleanness. You seek salvation, yet you have not followed its path, For a ship cannot sail on dry land. | Our      |
| وَكَانَتْ الْوَلَايَاتُ الْمُتَّحِدَةُ قَدْ أَعْلَنْتْ مِنْذُ أَيَّامٍ عَنْ اسْتِثْنَائِهَا لِسَبْعِ دُولٍ مِنَ الْعُقُوبَاتِ الَّتِي يَفْرِضُهَا " قَانُونُ إِقْرَارِ الدِّفَاعِ الْوَطَنِيِّ " لِسَنَةِ 2102 الصَّادِرِ فِي دَيْسَمِيرِ الْمَاضِي عَلَى شَرَكَاتِ الدُّوَلِ الَّتِي لَا تُخَفِّضُ وَارِدَاتِهَا مِنَ التَّقِطِ الْإِيرَانِيِّ بِشَكْلِ مَلْحُوظٍ مِنْ 82 يُونِيُو الْجَارِي، وَهَذَا الْاسْتِثْنَاءُ لَمْ يَشْمَلِ الصِّينَ.                                                                                                                         | The United States has recently announced an exemption for seven countries from the sanctions imposed by the "National Defense Authorization Act" issued last December on companies of countries that do not significantly reduce their imports of Iranian oil starting from June 28th, and this exemption did not include China.                                                                                                                                                                                             | WikiNews |

| Sample                                                                                                                                                                                                                                                                                                                                                                                                                                                                                                                                                                                                                                                                                                                                                                                                                                                                                                                                                                                                                                                                                                                                                                                                                                                 | Translation                                                                                                                                                                                                                                                                                                                                                                                                                                                                                                                                                                                                                                                                                                                                                                                                                                                                                                                                                                                                                                                                                                                                                                                                                                                                                                                                                                        | Source          |
|--------------------------------------------------------------------------------------------------------------------------------------------------------------------------------------------------------------------------------------------------------------------------------------------------------------------------------------------------------------------------------------------------------------------------------------------------------------------------------------------------------------------------------------------------------------------------------------------------------------------------------------------------------------------------------------------------------------------------------------------------------------------------------------------------------------------------------------------------------------------------------------------------------------------------------------------------------------------------------------------------------------------------------------------------------------------------------------------------------------------------------------------------------------------------------------------------------------------------------------------------------|------------------------------------------------------------------------------------------------------------------------------------------------------------------------------------------------------------------------------------------------------------------------------------------------------------------------------------------------------------------------------------------------------------------------------------------------------------------------------------------------------------------------------------------------------------------------------------------------------------------------------------------------------------------------------------------------------------------------------------------------------------------------------------------------------------------------------------------------------------------------------------------------------------------------------------------------------------------------------------------------------------------------------------------------------------------------------------------------------------------------------------------------------------------------------------------------------------------------------------------------------------------------------------------------------------------------------------------------------------------------------------|-----------------|
| <p>وَنَوَّهَ التَّقْرِيرُ إِلَى اِحْتِمَالِ أَنْ تَبْرَ بَعْضَ مَحَاصِلِ الْمَوْسِمِ الْجَارِي بِلَا حَصَادٍ نَتِجَةً تَزُوجُ السَّكَّانَ وَعَدَمِ تَوْفُرِ الْأَلَاتِ وَالْمَوَارِدِ وَالْوُقُودِ وَخَطَرِ الْعُنْفِ وَتَدْمِيرِ مَرَافِقِ التَّخْزِينِ. وَذَكَرَ التَّقْرِيرُ نَقْصَ اِئْتِاجِ الْحَبِيزِ فِي كُلِّ أَنْحَاءِ الْبِلَادِ.</p>                                                                                                                                                                                                                                                                                                                                                                                                                                                                                                                                                                                                                                                                                                                                                                                                                                                                                                        | <p>The report highlighted the possibility that some crops of the current season might be lost without harvest, due to population displacement, lack of machinery, resources, fuel, the danger of violence, and the destruction of storage facilities. The report also noted a shortage of bread production across the country.</p>                                                                                                                                                                                                                                                                                                                                                                                                                                                                                                                                                                                                                                                                                                                                                                                                                                                                                                                                                                                                                                                 | <p>WikiNews</p> |
| <p>كَمَا تَحَدَّثَ بِنَيَّامِينَ مَأْكُوْهَلٍ فِي مُحَاضَرَةٍ أُخْرَى عَنْ تَقْدِيمِ الْبَحْثِ الْعِلْمِيَّةِ الْمُتَعَلِّقَةِ بِوِيكِيبيديَا بَيْنَ عَامَيْ 2102 وَ 3102، وَتَنَاوُلِ عَيِّنَاتٍ مِنْ أَفْضَلِ وَأَشْمَلِ الْبَحْثِ الَّتِي خَصَّهَا وَدَقَّقَهَا، حَيْثُ كَانَ يَبْنِيهَا بِحَثٍ يَحُلُّ الطَّبِيعَةَ الْمَوْسُوعِيَّةَ لَوِيكِيبيديَا، وَآخِرُ يَتَنَاوَلُ مَشْرُوعَ وَيَكَمُوسِ الشَّقِيقِ، إِضَافَةً إِلَى أَرْبَعَةِ بَحْثٍ أُخْرَى.</p>                                                                                                                                                                                                                                                                                                                                                                                                                                                                                                                                                                                                                                                                                                                                                                                         | <p>Mackill in another lecture discussed the progress of scientific research related to Wikipedia between 2012 and 2013, and examined samples of the best and most comprehensive research he had reviewed and verified. Among these was a research paper analyzing the encyclopedic nature of Wikipedia, another addressing the Wikamouse sibling project, in addition to four other research papers.</p>                                                                                                                                                                                                                                                                                                                                                                                                                                                                                                                                                                                                                                                                                                                                                                                                                                                                                                                                                                           | <p>WikiNews</p> |
| <p>(قَوْلُهُ: وَلَوْ ادَّعَى وَلَدُ أُمَةٍ مُشْتَرَكَةً ثَبَتَ نَسَبُهُ، وَهِيَ أُمٌ وَلَدُهُ، وَلَزِمَهُ نَصْفُ قِيَمَتِهَا وَنَصْفُ عَقْرِهَا لَا قِيَمَتَهُ) أَمَّا ثُبُوتُ النَّسَبِ فَلأنَّهُ لَمَّا ثَبَتَ فِي نَصْفِهِ لِمَصَادِفَتِهِ مَلَكَةً ثَبَتَ فِي الْبَاقِي ضَرُورَةً أَنَّهُ لَا يَجْزَأُ لَمَّا أَنَّ سَبَبَهُ لَا يَجْزَأُ وَهُوَ الْعُلُوقُ إِذْ الْوَلَدُ الْوَاحِدُ لَا يَعْلقُ مِنْ مَاءَيْنِ، وَأَمَّا صِيرُورَتُهَا أُمٌ وَلَدُ فَلَانِ الْإِسْتِيلَادِ لَا يَجْزَأُ عِنْدَهُ وَعِنْدَهُمَا يَصِيرُ نَصِيبُهُ أُمٌ وَلَدُ لَهُ، ثُمَّ يَمْلِكُ نَصِيبَ صَاحِبِهِ إِذْ هُوَ قَابِلٌ لِلْمَلِكِ، وَأَمَّا ضَمَانُ نَصْفِ الْقِيَمَةِ فَلأنَّهُ تَمْلِكُ نَصِيبَ صَاحِبِهِ لَمَّا اسْتَكْمَلَ الْإِسْتِيلَادَ، وَأَمَّا ضَمَانُ نَصْفِ الْعَقْرِ فَلأنَّهُ وَطِئَ جَارِيَةً مُشْتَرَكَةً إِذْ الْمَلِكُ ثَبَتَ حَكْمًا لِلْإِسْتِيلَادِ فَيَعْقِبُهُ الْمَلِكُ فِي نَصِيبِ صَاحِبِهِ بِخِلَافِ الْأَبِ؛ إِذَا اسْتَوْلَدَ جَارِيَةً ابْنَهُ؛ لِأَنَّ الْمَلِكَ هُنَاكَ ثَبَتَ شَرْطًا لِلْإِسْتِيلَادِ فَيَتَقَدَّمُهُ فَصَارَ وَأَطْلًا مَلِكٌ نَفْسِهِ، وَأَمَّا عَدَمُ ضَمَانِ قِيَمَةِ الْوَلَدِ فَلأنَّ النَّسَبَ يَثْبُتُ مُسْتَنَدًا إِلَى وَقْتِ الْعُلُوقِ فَلَمْ يَتَعَلَّقْ شَيْءٌ مِنْهُ عَلَى مَلِكٍ شَرِيكِهِ.</p> | <p>”(His statement: If a co-owned slave’s child claims lineage, his lineage is established, and she becomes his mother, and he is liable for half her value and half her compensation)<br/>Regarding the establishment of lineage: Since it was proven in half due to matching his ownership, it is established in the remainder necessarily, as lineage cannot be divided, because its cause (conception) is indivisible - a single child cannot be conceived from two different waters.<br/>Regarding her becoming a ‘mother of a child’: Procreation is indivisible, so his share becomes his ‘mother of a child’, and then he can acquire his partner’s share as it is transferable. Regarding the guarantee of half her value: He acquired his partner’s share after completing procreation. Regarding the guarantee of half the compensation: He had sexual relations with a co-owned slave girl, as ownership is legally established through procreation, which is followed by ownership of his partner’s share. This differs from a father who impregnates his son’s slave, where ownership is a conditional prerequisite for procreation, making him effectively an owner of his own property. Regarding non-liability for the child’s value: Lineage is established retroactively to the time of conception, so nothing is claimed against his partner’s ownership.”</p> | <p>Fadel</p>    |

| Sample                                                                                                                                                                                                                                                                                                                                                                                                                                                                                                                                                                                                                                                                                                                                                                                                                                                                                            | Translation                                                                                                                                                                                                                                                                                                                                                                                                                                                                                                                                                                                                                                                                                                                                                                                                                                                                                    | Source       |
|---------------------------------------------------------------------------------------------------------------------------------------------------------------------------------------------------------------------------------------------------------------------------------------------------------------------------------------------------------------------------------------------------------------------------------------------------------------------------------------------------------------------------------------------------------------------------------------------------------------------------------------------------------------------------------------------------------------------------------------------------------------------------------------------------------------------------------------------------------------------------------------------------|------------------------------------------------------------------------------------------------------------------------------------------------------------------------------------------------------------------------------------------------------------------------------------------------------------------------------------------------------------------------------------------------------------------------------------------------------------------------------------------------------------------------------------------------------------------------------------------------------------------------------------------------------------------------------------------------------------------------------------------------------------------------------------------------------------------------------------------------------------------------------------------------|--------------|
| <p>كَهَيْلٍ قَالَ سَمِعْتُ أَبِي يُحَدِّثُ عَنْ حَبَّةِ الْعَرْنِيِّ قَالَ رَأَيْتُ عَلِيًّا رَضِيَ اللَّهُ عَنْهُ ضَحَكَ عَلَى الْمَنْبَرِ لَمْ أَرَهُ ضَحَكَ ضَحْكًا أَكْثَرَ مِنْهُ حَتَّى بَدَتْ نَوَاجِذُهُ ثُمَّ قَالَ ذَكَرْتُ قَوْلَ أَبِي طَالِبٍ ظَهَرَ عَلَيْنَا أَبُو طَالِبٍ وَأَنَا مَعَ رَسُولِ اللَّهِ صَلَّى اللَّهُ عَلَيْهِ وَسَلَّمَ وَنَحْنُ نَصِيٌّ بِبَطْنِ نَخْلَةٍ فَقَالَ مَاذَا تَصْنَعَانِ يَا ابْنَ أَخِي فَدَعَاهُ رَسُولُ اللَّهِ صَلَّى اللَّهُ عَلَيْهِ وَسَلَّمَ إِلَى الْإِسْلَامِ فَقَالَ مَا بِالَّذِي تَصْنَعَانِ بِأَسْ أَوْ بِالَّذِي تَقُولَانِ بِأَسْ وَلَكِنْ وَاللَّهِ لَا تَعْلَوْنِي اسْتَبَدَّ أَبَدًا وَضَحَكَ تَعَجُّبًا لِقَوْلِ أَبِيهِ ثُمَّ قَالَ اللَّهُمَّ لَا أَعْرِفُ أَنَّ عَبْدًا لَكَ مِنْ هَذِهِ الْأُمَّةِ عَبْدُكَ قَبْلِي غَيْرَ نَبِيِّكَ ثَلَاثَ مَرَّاتٍ لَقَدْ صَلَّيْتُ قَبْلَ أَنْ يُصَلِّيَ النَّاسُ سَبْعًا (661 / 2)</p> | <p>Narrated by Habba Al-Urani: He said, "I saw Ali (may Allah be pleased with him) laughing on the pulpit in a way I had never seen him laugh before, until his molars became visible. Then he said: I remembered the words of Abu Talib when he approached us while I was with the Messenger of Allah (peace be upon him), and we were praying in the valley of Nakhla. He said, 'What are you doing, my nephew?' The Messenger of Allah invited him to Islam, and he responded, 'There is no harm in what you are doing or in what you are saying. But by Allah, you will never overcome me.' He (Ali) laughed in amazement at his father's words, then said, 'O Allah, I do not acknowledge any of Your servants from this nation who worshipped You before me, except Your Prophet,' repeating this three times. (He then added) 'I prayed seven times before people started praying.'</p> | <p>Fadel</p> |
| <p>بِأَنَّهُمْ يَقْرَأُونَ الْقُرْآنَ لَا يَجَاوِزُ تَرَاقِيَهُمْ، يَعْنِي وَاللَّهِ أَعْلَمُ أَنَّهُمْ لَا يَنْتَفَهُونَ بِهِ حَتَّى يَصِلَ إِلَى قُلُوبِهِمْ لِأَنَّ الْفَهْمَ رَاجِعٌ إِلَى الْقَلْبِ، فَإِذَا لَمْ يَصِلْ إِلَى الْقَلْبِ لَمْ يَحْصُلْ فِيهِ فَهْمٌ عَلَى حَالٍ، وَإِنَّمَا يَقِفُ عِنْدَ مَحَلِّ الْأَصْوَاتِ وَالْحُرُوفِ الْمَسْمُوعَةِ فَقَطْ، وَهُوَ الَّذِي يَشْتَرِكُ فِيهِ مَنْ يَفْهَمُ وَمَنْ لَا يَفْهَمُ، وَمَا تَقْدَمُ أَيْضًا مِنْ قَوْلِهِ عَلَيْهِ الصَّلَاةُ وَالسَّلَامُ: إِنَّ اللَّهَ لَا يَقْبِضُ الْعِلْمَ انْتِزَاعًا إِلَى آخِرِهِ.</p>                                                                                                                                                                                                                                                                                                             | <p>They recite the Quran, but it does not pass beyond their throats, meaning - and Allah knows best - that they do not understand it deeply enough for it to reach their hearts, because understanding returns to the heart. If it does not reach the heart, no true comprehension will occur at all. Instead, it remains at the level of heard sounds and letters, which is something shared by those who understand and those who do not understand. This is also supported by his (peace be upon him) previous statement: 'Indeed, Allah does not withdraw knowledge suddenly...' (continuing to the end of the hadith)</p>                                                                                                                                                                                                                                                                 | <p>Fadel</p> |
